# Supplementary material for: Fermionic multicriticality near Kekul\'{e} valence-bond ordering in honeycomb lattice
Source: arXiv:1902.08616 source file (2019-06-05)
Supplement: Supplementary file 1 [file Supplementary_KekuleMCP.pdf]

# Supplementary Materials: Fermionic multicriticality near Kekulé valence-bond ordering in honeycomb lattice

Bitan Roy[1] and Vladimir Juričić[2]

[1]Max-Planck-Institut für Physik komplexer Systeme, Nöthnitzer Stra. 38, 01187 Dresden, Germany
[2]Nordita, KTH Royal Institute of Technology and Stockholm University, Roslagstullsbacken 23, 10691 Stockholm, Sweden

In this Supplementary Materials (SM) we present the details of the diagramatic analysis of the effective coupled Gross-Neveu-Yukawa model in the presence of all symmetry allowed cubic terms. Recall that the corresponding imaginary time ($\tau$) action reads as $\mathcal{S} = \int d\tau d^d \boldsymbol{r} L$, with $L = L_f + L_{bf} + L_b$ and $\boldsymbol{r} = (x_1, \cdots, x_d)$ is the spatial coordinate. Various components of $L$ are

$$L_f = \Psi^\dagger(\tau, \mathbf{r}) \left[ \partial_\tau - i \sum_{j=1}^{d} \Gamma_j \partial_j \right] \Psi(\tau, \mathbf{r}), \quad L_{bf} = \sum_{j=1}^{2} g_j \Phi_j \Psi^\dagger M_j \Psi + g_3 \sum_{k=1}^{N_b} \chi_k \Psi^\dagger M_{2+k} \Psi, \tag{1}$$

and $L_b = L_{\rm Kek} + L^{N_b}_{\rm Sym} + L_{\rm Mix}$, where

$$L_{\rm Kek} = \sum_{j=1}^{2} \left[ \frac{1}{2} \left( \partial_\mu \Phi_j \right)^2 + m_j^2 \Phi_j^2 \right] + \frac{u_1}{3!} \Phi_1^3 + \frac{u_2}{2!} \Phi_1 \Phi_2^2 + \sum_{j=1}^{2} \frac{\lambda_j}{4!} \Phi_j^4 + \frac{2\lambda_{12}}{4!} \Phi_1^2 \Phi_2^2,$$
$$L^{N_b}_{\rm Sym} = \sum_{j=1}^{N_b} \left[ \frac{1}{2} \left( \partial_\mu \chi_j \right)^2 + m_3^2 \chi_j^2 + \frac{\lambda_3}{4!} \left( \chi_j^2 \right)^2 \right], \quad L_{\rm Mix} = \frac{u_3}{2!} \Phi_1 \sum_{j=1}^{N_b} \chi_j^2 + \left( \sum_{j=1}^{2} \frac{2\lambda_{j3}}{4!} \Phi_j^2 \right) \sum_{k=1}^{N_b} \chi_j^2. \tag{2}$$

Notations are already introduced in the main part of the paper. We here only present the details of the leading order perturbative renormalization group (RG) analysis of the above model.

## A. Bosonic self-energy correction

The leading order self-energy correction for the $\Phi_1$ field arises from Feynman diagrams (a)-(d) of Fig. 1. The total contribution from these diagrams is given by

$$\text{Con}^{(1)}_{\rm (a)-(d)} = -(\omega^2 + \mathbf{q}^2) \left[ 2 N_f g_1^2 \frac{\Lambda^{D-4}}{8\pi^2} + \frac{1}{6} \left( u_1^2 + u_2^2 + N_b u_3^2 \right) \frac{\Lambda^{D-6}}{8\pi^2} \right] \ell, \tag{3}$$

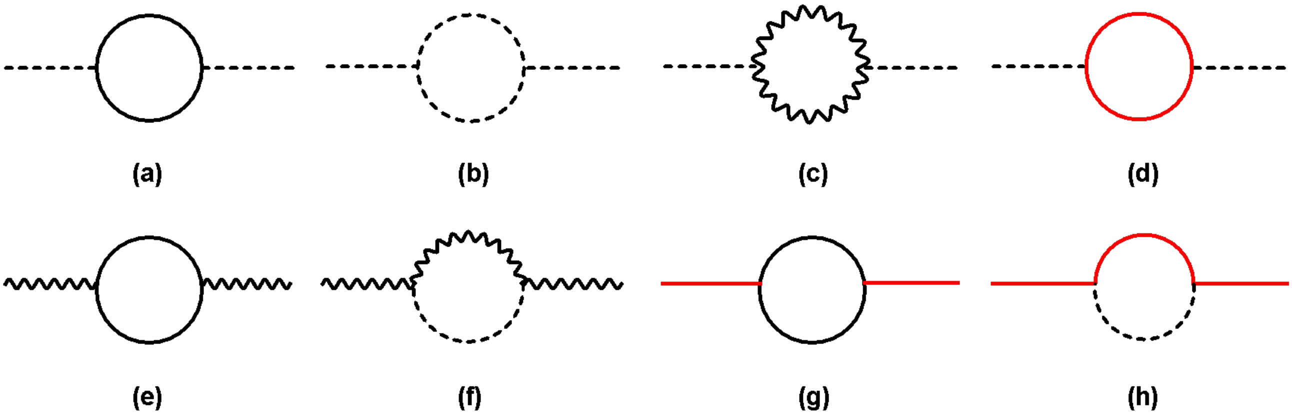


Figure 1: Feynman diagrams contributing to the self-energy of three bosonic fields. Here solid black lines represent massless Dirac fermions. By contrast, dashed, wavy and red lines respectively represent $\Phi_1$, $\Phi_2$ and $\chi$ bosonic fields. We follow the same notation for all the remaining figures in this Supplemental Materials.

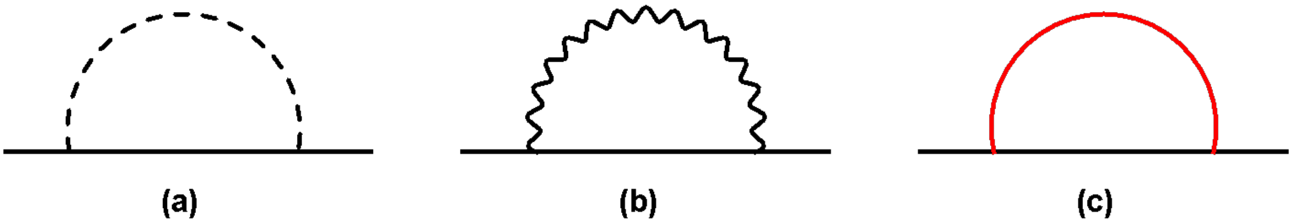


Figure 2: Feynman diagrams contributing to the self-energy of Dirac fermions due to three Yukawa couplings.

where $D = d + 1$ is the space-(imaginary)time dimensions, $\Lambda$ is the ultraviolet momentum cutoff, $\ell$ is the logarithm of the renormalization group scale, $\omega$ and $\mathbf{q}$ are respectively the external frequency and momentum of bosonic field $\Phi_1$. The self-energy correction of $\Phi_2$ and $\boldsymbol{\chi}$ fields respectively arises from diagrams (e), (f) and (g), (h). Respectively, the net contributions from these two sets of diagrams are given by

$$\text{Con}^{(1)}_{(\text{e})-(\text{f})} = -(\omega^2 + \mathbf{q}^2) \left[ 2N_f g_2^2 \frac{\Lambda^{D-4}}{8\pi^2} + \frac{1}{3} u_2^2 \frac{\Lambda^{D-6}}{8\pi^2} \right] \ell, \quad \text{Con}^{(1)}_{(\text{g})-(\text{h})} = -(\omega^2 + \mathbf{q}^2) \left[ 2N_f g_3^2 \frac{\Lambda^{D-4}}{8\pi^2} + \frac{1}{3} u_3^2 \frac{\Lambda^{D-6}}{8\pi^2} \right] \ell, \quad (4)$$

The bosonic field renormalization factors are then given by

$$Z_{\Phi_1} = 1 - 2N_f g_1^2 \ell - \frac{1}{6} \left( u_1^2 + u_2^2 + N_b u_3^2 \right) \ell, \quad Z_{\Phi_2} = 1 - 2N_f g_2^2 \ell - \frac{1}{3} u_2^2 \ell, \quad Z_{\boldsymbol{\chi}} = 1 - 2N_f g_3^2 \ell - \frac{1}{3} u_3^2 \ell, \quad (5)$$

in terms of dimensionless coupling constants, defined as $g_j^2 \Lambda^{D-4}/(8\pi^2) \to g_j^2$ and $u_j^2 \Lambda^{D-6}/(8\pi^2) \to u_j^2$, for $j = 1, 2, 3$.

## B. Fermionic self-energy correction

The leading order self-energy correction for massless Dirac fermions arises from Feynman diagrams (a)-(c), shown in Fig. 2. The net contribution from these three diagrams is given by

$$\text{Con}^{(2)}_{(\text{a})-(\text{c})} = i(\omega + \Gamma_j q_j) \, \frac{1}{2} \left[ g_1^2 + g_2^2 + N_b g_3^2 \right] \frac{\Lambda^{D-4}}{8\pi^2} \, \ell, \quad (6)$$

yielding the fermionic field renormalization ($Z_\Psi$)

$$Z_\Psi = 1 - \frac{1}{2} \left( g_1^2 + g_2^2 + N_b g_3^2 \right) \ell, \quad (7)$$

in terms of dimensionless Yukawa couplings.

## C. Renormalization of Yukawa vertices

The renormalization of three Yukawa vertices $g_1$, $g_2$ and $g_3$, respectively arises from diagrams (a)-(c), (d)-(f) and (g)-(i) of Fig. 3. Contributions from these three sets of Feynman diagrams are respectively given by

$$\begin{aligned} \text{Con}^{(3)}_{(\text{a})-(\text{c})} &= \left[ -g_1^2 + g_2^2 + N_b g_3^2 \right] \frac{\Lambda^{D-4}}{8\pi^2} \, \ell, \\ \text{Con}^{(3)}_{(\text{d})-(\text{f})} &= \left[ g_1^2 - g_2^2 + N_b g_3^2 \right] \frac{\Lambda^{D-4}}{8\pi^2} \, \ell, \\ \text{Con}^{(3)}_{(\text{g})-(\text{i})} &= \left[ g_1^2 + g_2^2 + (N_b - 2) \, g_3^2 \right] \frac{\Lambda^{D-4}}{8\pi^2} \, \ell. \end{aligned} \quad (8)$$

The renormalization group flow equations for $g_1^2$, $g_2^2$ and $g_3^2$ can respectively be obtained from the following conditions

$$Z_\Psi Z_{\Phi_1}^{1/2} g_{1,\text{B}} + g_{1,\text{B}} \text{Con}^{(3)}_{(\text{a})-(\text{c})} = g_{1,\text{R}}, \; Z_\Psi Z_{\Phi_2}^{1/2} g_{2,\text{B}} + g_{2,\text{B}} \text{Con}^{(3)}_{(\text{d})-(\text{f})} = g_{2,\text{R}}, \; Z_\Psi Z_{\boldsymbol{\chi}}^{1/2} g_{3,\text{B}} + g_{3,\text{B}} \text{Con}^{(3)}_{(\text{g})-(\text{i})} = g_{3,\text{R}}, \quad (9)$$

where the quantities with subscript 'B' and 'R' respectively stand for the bare and renormalized coupling constants. The resulting flow equations are shown in the main part of the paper [see Eq. (6)].

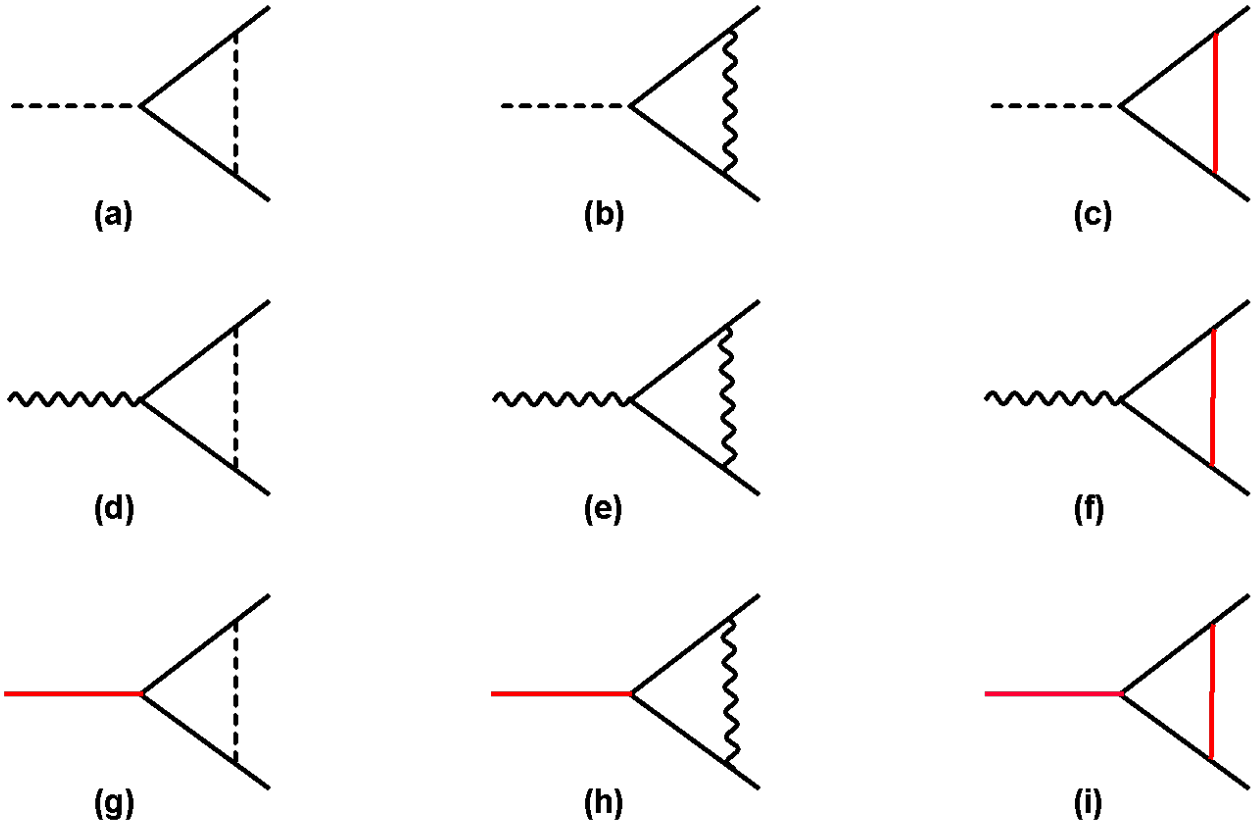


Figure 3: Feynman diagrams renormalizing three Yukawa vertices to the leading order. Namely, diagrams (a)-(c), (d)-(f) and (g)-(i) respectively renormalize Yukawa couplings $g_1$, $g_2$ and $g_3$, respectively.

### D. Renormalization of cubic vertices

• **Renormalization of** $u_1$: Feynman diagrams renormalizing the cubic vertex $u_1$ are shown in Fig. 4. The net contribution from the traingle diagrams [(a)-(c)] is given by

$$\text{Con}^{(4)}_{(a)-(c)} = -\frac{3!}{2}\left[u_1^3 + u_2^3 + N_b u_3^3\right] \frac{\Lambda^{D-6}}{8\pi^2}\,\ell. \tag{10}$$

On the other hand, the total contribution from the diagrams involving bosonic bubble [(d)-(f)] is given by

$$\text{Con}^{(4)}_{(d)-(f)} = \left[\frac{3}{2}u_1\lambda_1 + \frac{1}{2}u_2\lambda_{12} + \frac{N_b}{2}u_3\lambda_{13}\right] \frac{\Lambda^{D-4}}{8\pi^2}\,\ell. \tag{11}$$

The renormalization condition for $u_1$ is then given by

$$Z^{3/2}_{\Phi_1} u_{1,\mathrm{B}} + \text{Con}^{(4)}_{(a)-(c)} + \text{Con}^{(4)}_{(d)-(f)} = u_{1,\mathrm{R}}, \tag{12}$$

from which we obtain the RG flow equation for $u_1$, shown in the main part of the paper [see Eq. (6)].

• **Renormalization of** $u_2$: Feynman diagrams renormalizing the cubic vertex $u_2$ are shown in Fig. 5. The net contribution from the triangle diagrams [(a), (b)] is given by

$$\text{Con}^{(5)}_{(a)-(b)} = -\left[u_1 u_2^2 + u_2^3\right] \frac{\Lambda^{D-6}}{8\pi^2}\,\ell. \tag{13}$$

The total contribution from diagrams (c)-(f) of Fig. 5 is given by

$$\text{Con}^{(5)}_{(c)-(f)} = \left[u_2\lambda_2 + \frac{1}{3}u_1\lambda_{12} + \frac{1}{3}u_2\lambda_{12} + \frac{N_b}{3}u_3\lambda_{23}\right] \frac{\Lambda^{D-4}}{8\pi^2}\,\ell. \tag{14}$$

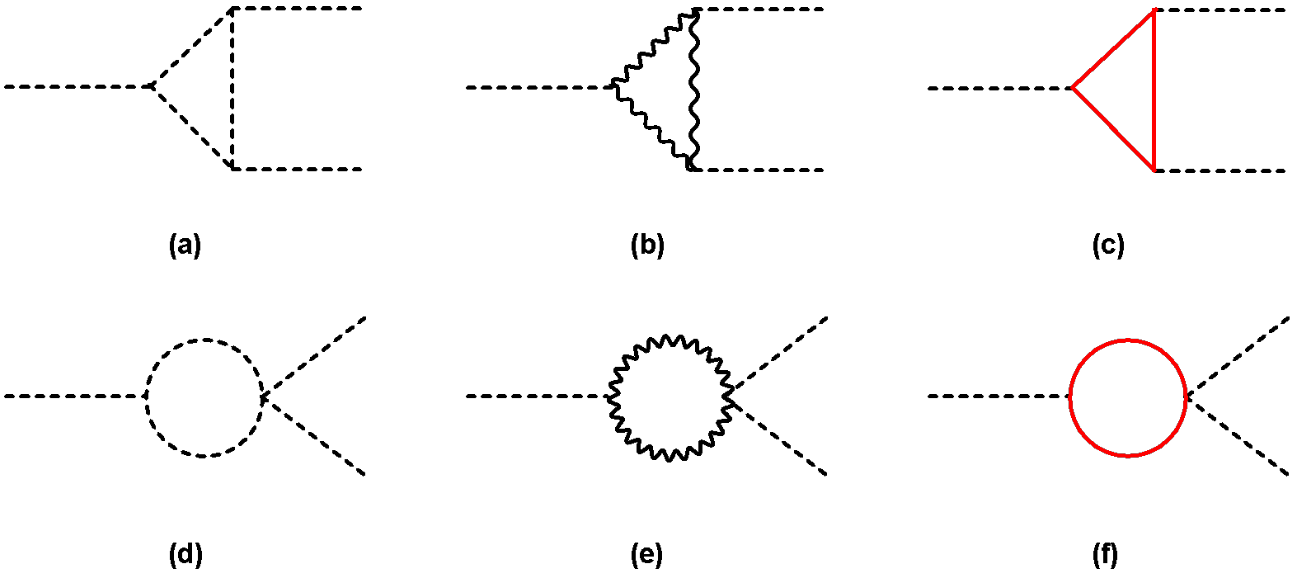


Figure 4: Feynman diagrams renormalizing cubic vertex $u_1$ to the leading order.

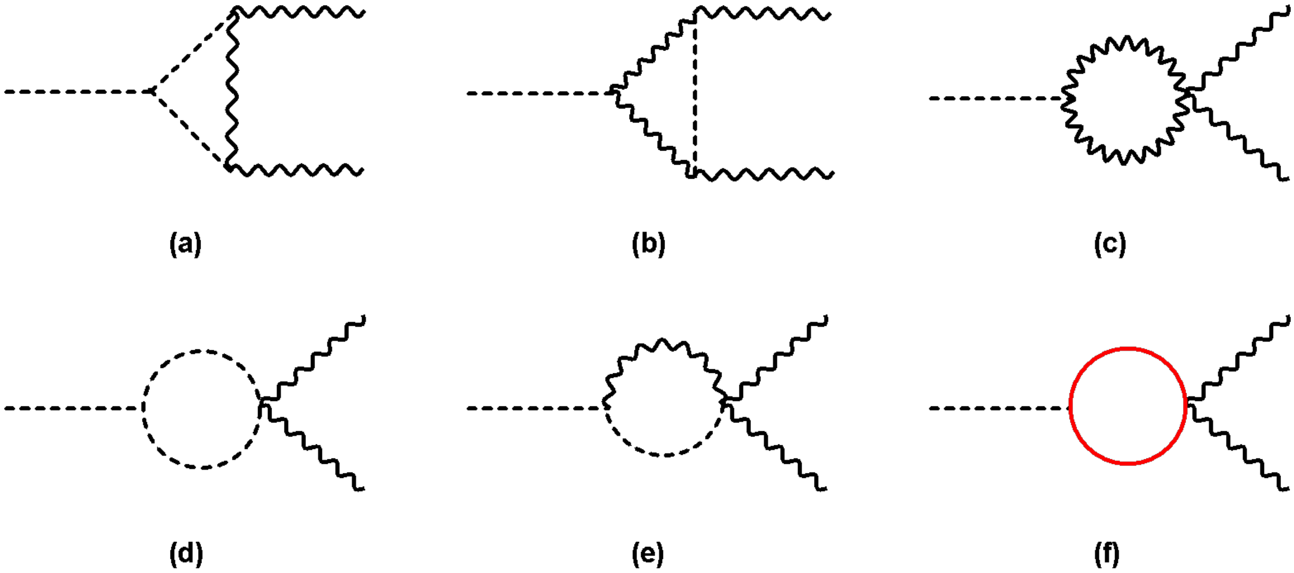


Figure 5: Feynman diagrams renormalizing cubic vertex $u_2$ to the leading order.

The renormalization condition for $u_2$ is then given by

$$Z_{\Phi_1}^{1/2} Z_{\Phi_2} u_{2,\mathrm{B}} + \mathrm{Con}^{(5)}_{(\mathrm{a})-(\mathrm{b})} + \mathrm{Con}^{(5)}_{(\mathrm{c})-(\mathrm{f})} = u_{2,\mathrm{R}}, \tag{15}$$

from which we obtain the RG flow equation for $u_2$, shown in the main part of the paper [see Eq. (6)].

• **Renormalization of $u_3$**: Feynman diagrams renormalizing the cubic vertex $u_3$ are shown in Fig. 6. The net contribution from the triangle diagram [(a), (b)] reads

$$\mathrm{Con}^{(6)}_{(\mathrm{a})-(\mathrm{b})} = -\left[u_1 u_3^2 + u_3^3\right] \frac{\Lambda^{D-6}}{8\pi^2} \ell. \tag{16}$$

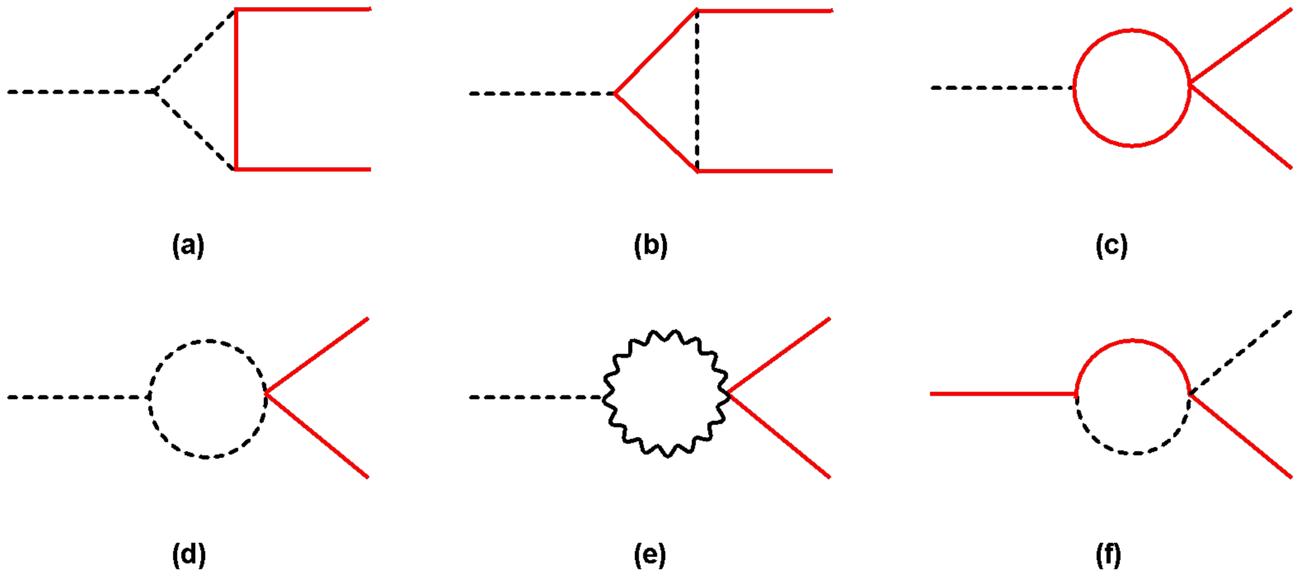


Figure 6: Feynman diagrams renormalizing cubic vertex $u_3$ to the leading order.

The total contribution from diagrams (c)-(f) of Fig. 6 is given by

$$\mathrm{Con}^{(6)}_{(\mathrm{c})-(\mathrm{f})} = \left[\frac{1}{3}\left(N_b+2\right) u_3 \lambda_3 + \frac{1}{3} u_1 \lambda_{13} + \frac{1}{3} u_2 \lambda_{23} + \frac{1}{3} u_3 \lambda_{13}\right] \frac{\Lambda^{D-4}}{8\pi^2}\, \ell. \tag{17}$$

The renormalization condition for $u_3$ is then given by

$$Z^{1/2}_{\Phi_1} Z_{\boldsymbol{\chi}} u_{3,\mathrm{B}} + \mathrm{Con}^{(6)}_{(\mathrm{a})-(\mathrm{b})} + \mathrm{Con}^{(6)}_{(\mathrm{c})-(\mathrm{f})} = u_{3,\mathrm{R}}, \tag{18}$$

from which we obtain the RG flow equation for $u_3$, shown in the main part of the paper [see Eq. (6)].

### E. Renormalization of quartic boson couplings

• **Renormalization of** $\lambda_1$: The leading order renormalization of quartic bosonic coupling $\lambda_1$ arises from the Feynman diagrams shown in Fig. 7. The net contribution from diagrams (a)-(c) is given by

$$\mathrm{Con}^{(7)}_{(\mathrm{a})-(\mathrm{c})} = \left[\frac{3}{2}\lambda_1^2 + \frac{1}{6}\lambda_{12}^2 + \frac{N_b}{6}\lambda_{13}^2\right] \frac{\Lambda^{D-4}}{8\pi^2}\, \ell. \tag{19}$$

The net contribution from diagrams (d)-(g) is given by

$$\mathrm{Con}^{(7)}_{(\mathrm{d})-(\mathrm{g})} = -24 N_f g_1^4 \,\frac{\Lambda^{D-4}}{8\pi^2} \ell + 12\left[u_1^4 + u_1^4 + N_b u_3^4\right] \frac{\Lambda^{D-8}}{8\pi^2}\, \ell. \tag{20}$$

The net contribution from diagrams (h)-(j) is given by

$$\mathrm{Con}^{(7)}_{(\mathrm{h})-(\mathrm{i})} = -\left[12\lambda_1 u_1^2 + 4\lambda_{12} u_2^2 + 4 N_b \lambda_{13} u_3^2\right] \frac{\Lambda^{D-6}}{8\pi^2}\, \ell. \tag{21}$$

The renormalization condition for $\lambda_1$ then reads as

$$Z^2_{\Phi_1}\lambda_{1,\mathrm{B}} - \mathrm{Con}^{(7)}_{(\mathrm{a})-(\mathrm{c})} - \mathrm{Con}^{(7)}_{(\mathrm{d})-(\mathrm{g})} - \mathrm{Con}^{(7)}_{(\mathrm{h})-(\mathrm{i})} = \lambda_{1,\mathrm{R}}, \tag{22}$$

from which we arrive at the RG flow equation for $\lambda_1$ quoted in the main part of the paper [see Eq. (6)].

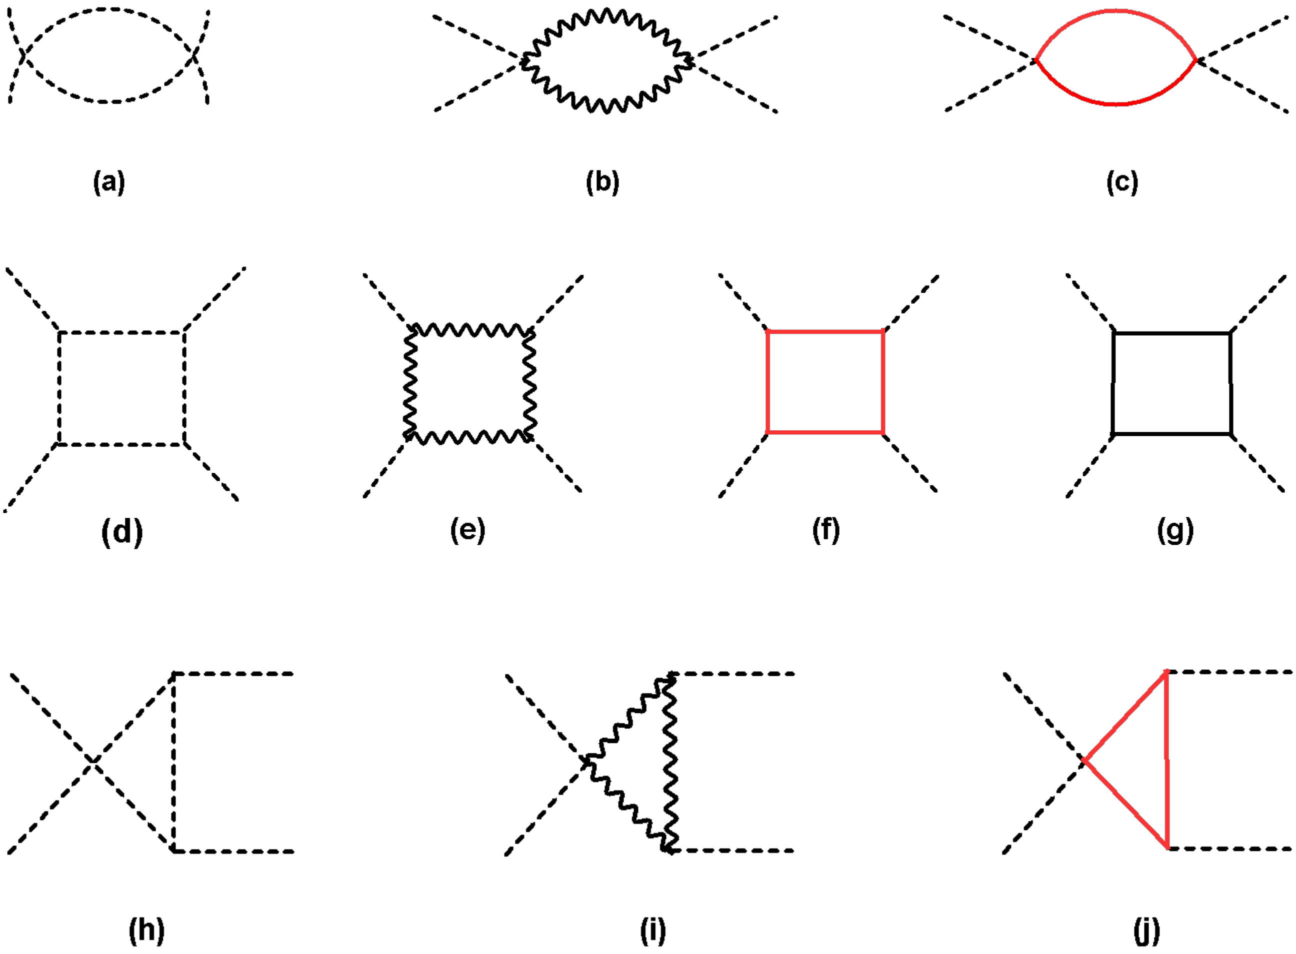


Figure 7: Feynman diagrams renormalizing quartic bosnic interaction $\lambda_1$ to the leading order.

• **Renormalization of** $\lambda_2$: The leading order renormalization of quartic bosonic coupling $\lambda_2$ arises from the Feynman diagrams shown in Fig. 8. The net contribution from diagrams (a)-(c) is given by

$$\text{Con}^{(8)}_{(\text{a})-(\text{c})} = \left[\frac{3}{2}\lambda_2^2 + \frac{1}{6}\lambda_{12}^2 + \frac{N_b}{6}\lambda_{23}^2\right] \frac{\Lambda^{D-4}}{8\pi^2} \, \ell. \tag{23}$$

The net contribution from diagrams (d) and (e) is given by

$$\text{Con}^{(8)}_{(\text{d})-(\text{e})} = -24 N_f g_2^4 \, \frac{\Lambda^{D-4}}{8\pi^2} \ell + 24 u_{_2}^4 \, \frac{\Lambda^{D-8}}{8\pi^2} \, \ell. \tag{24}$$

The net contribution from diagrams (f) and (g) is given by

$$\text{Con}^{(8)}_{(\text{f})-(\text{g})} = -\left[12\lambda_2 u_{_2}^2 + 4\lambda_{12} u_{_2}^2\right] \frac{\Lambda^{D-6}}{8\pi^2} \, \ell. \tag{25}$$

The renormalization condition for $\lambda_2$ then reads as

$$Z^2_{\Phi_2} \lambda_{2,\text{B}} - \text{Con}^{(8)}_{(\text{a})-(\text{c})} - \text{Con}^{(8)}_{(\text{d})-(\text{e})} - \text{Con}^{(8)}_{(\text{f})-(\text{g})} = \lambda_{2,\text{R}}, \tag{26}$$

from which we arrive at the RG flow equation for $\lambda_2$ quoted in the main part of the paper [see Eq. (6)].

• **Renormalization of** $\lambda_3$: The leading order renormalization of quartic bosonic coupling $\lambda_3$ arises from the Feynman diagrams shown in Fig. 9. The net contribution from diagrams (a)-(c) is given by

$$\text{Con}^{(9)}_{(\text{a})-(\text{c})} = \left[\frac{1}{6}\left(N_b + 8\right)\lambda_3^2 + \frac{1}{6}\lambda_{13}^2 + \frac{1}{6}\lambda_{23}^2\right] \frac{\Lambda^{D-4}}{8\pi^2} \, \ell. \tag{27}$$

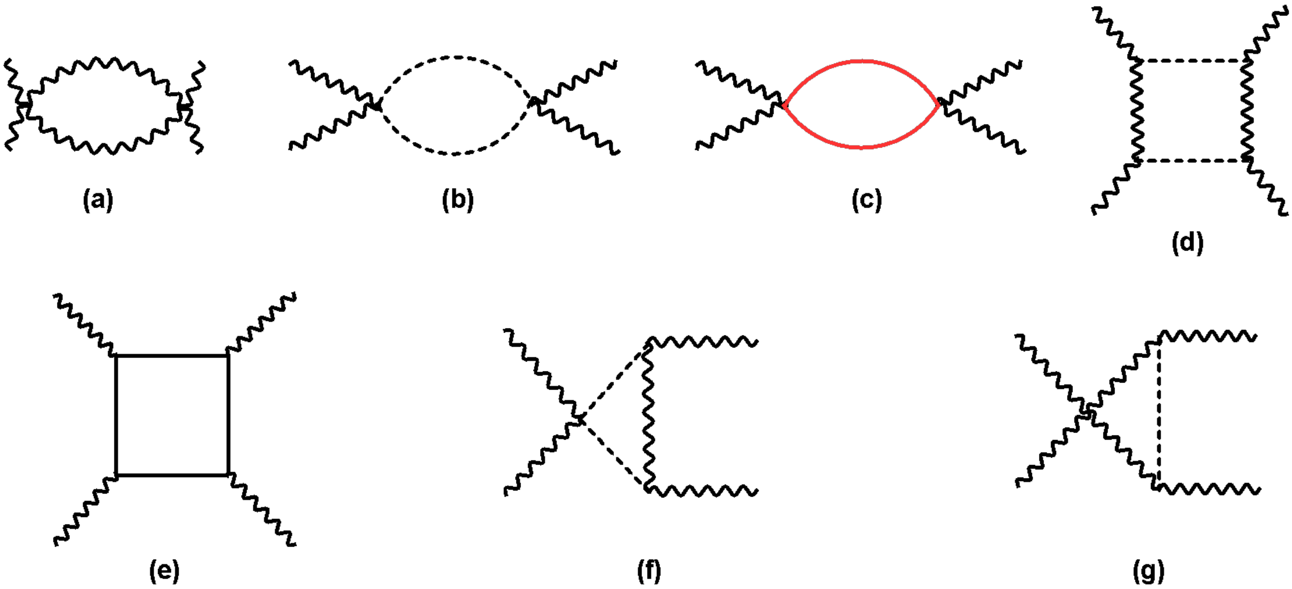


Figure 8: Feynman diagrams renormalizing quartic bosnic interaction $\lambda_2$ to the leading order.

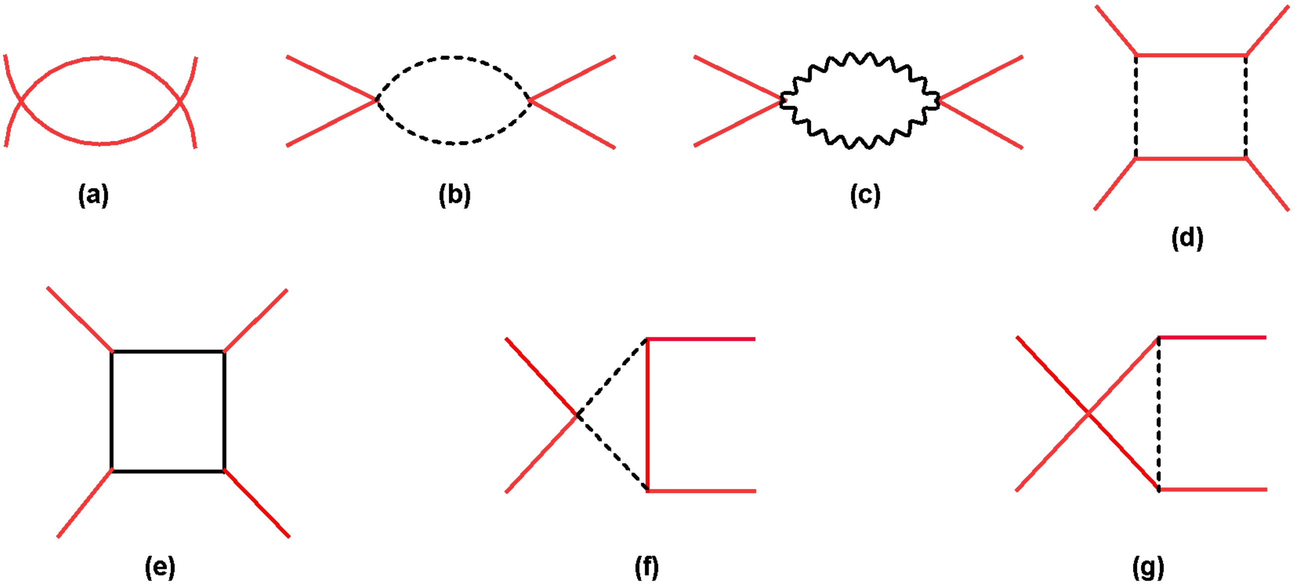


Figure 9: Feynman diagrams renormalizing quartic bosnic interaction $\lambda_3$ to the leading order.

The net contribution from diagrams (d) and (e) is given by

$$\text{Con}^{(9)}_{(\text{d})-(\text{e})} = -24 N_f g_3^4 \, \frac{\Lambda^{D-4}}{8\pi^2} \ell + 24 u_3^4 \, \frac{\Lambda^{D-8}}{8\pi^2} \, \ell. \tag{28}$$

The net contribution from diagrams (f) and (g) is given by

$$\text{Con}^{(9)}_{(\text{f})-(\text{g})} = -\left[12\lambda_3 u_3^2 + 4\lambda_{13} u_3^2\right] \, \frac{\Lambda^{D-6}}{8\pi^2} \, \ell. \tag{29}$$

The renormalization condition for $\lambda_3$ then reads as

$$Z_\chi^2 \lambda_{3,\text{B}} - \text{Con}^{(9)}_{(\text{a})-(\text{c})} - \text{Con}^{(9)}_{(\text{d})-(\text{e})} - \text{Con}^{(9)}_{(\text{f})-(\text{g})} = \lambda_{3,\text{R}}, \tag{30}$$

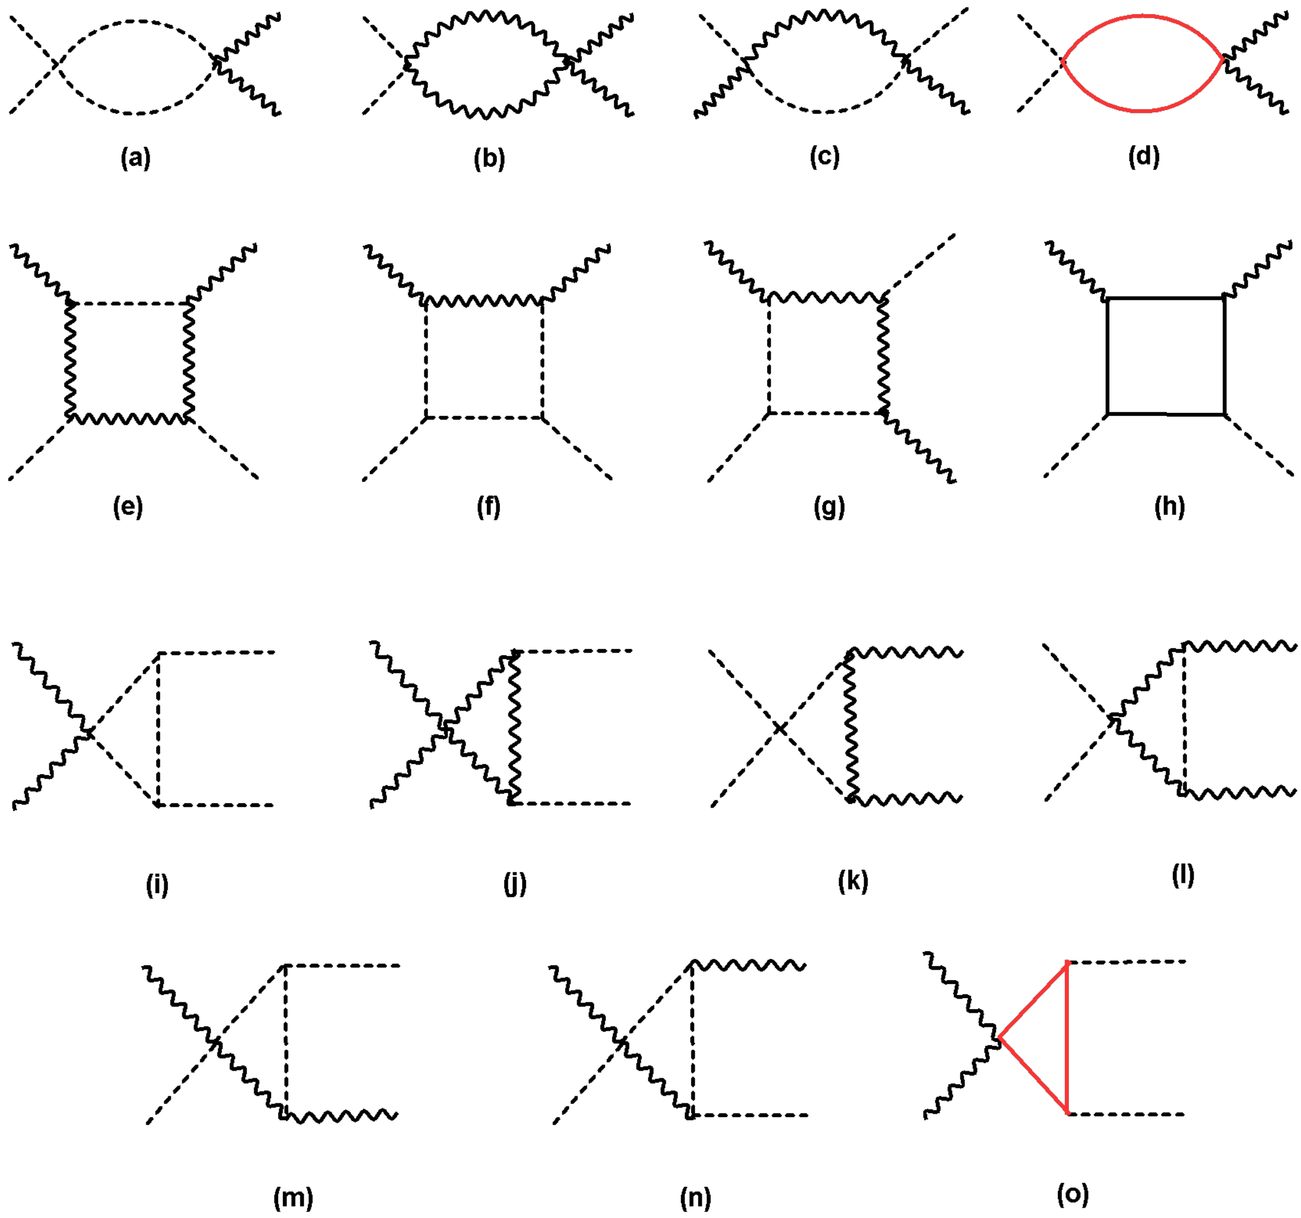


Figure 10: Feynman diagrams renormalizing quartic bosnic interaction $\lambda_{12}$ to the leading order.

from which we arrive at the RG flow equation for $\lambda_3$ quoted in the main part of the paper [see Eq. (6)].

• **Renormalization of** $\lambda_{12}$: The leading order renormalization of quartic bosonic coupling $\lambda_{12}$ arises from the Feynman diagrams shown in Fig. 10. The net contribution from diagrams (a)-(d) is given by

$$\text{Con}^{(10)}_{(\text{a})-(\text{d})} = \left[\frac{1}{6}\lambda_1\lambda_{12} + \frac{1}{6}\lambda_2\lambda_{12} + \frac{2}{9}\lambda_{12}^2 + \frac{N_b}{18}\lambda_{13}\lambda_{23}\right] \frac{\Lambda^{D-4}}{8\pi^2}\,\ell. \tag{31}$$

The net contribution from diagrams (e)-(h) is given by

$$\text{Con}^{(10)}_{(\text{e})-(\text{h})} = -8N_f g_1^2 g_2^2 \,\frac{\Lambda^{D-4}}{8\pi^2}\ell + \left[8u_2^4 + 8u_1^2 u_2^2 + 8u_1 u_2^3\right] \frac{\Lambda^{D-8}}{8\pi^2}\,\ell. \tag{32}$$

The net contribution from diagrams (i)-(o) is given by

$$\text{Con}^{(10)}_{(\text{i})-(\text{o})} = -\left[\frac{2}{3}\lambda_{12}u_1^2 + 2\lambda_2 u_2^2 + 2\lambda_1 u_2^2 + \frac{2}{3}\lambda_{12}u_2^2 + \frac{4}{3}\lambda_{12}u_1 u_2 + \frac{4}{3}\lambda_{12}u_2^2 + \frac{2}{3}N_b\lambda_{23}u_3^2\right] \frac{\Lambda^{D-6}}{8\pi^2}\,\ell. \tag{33}$$

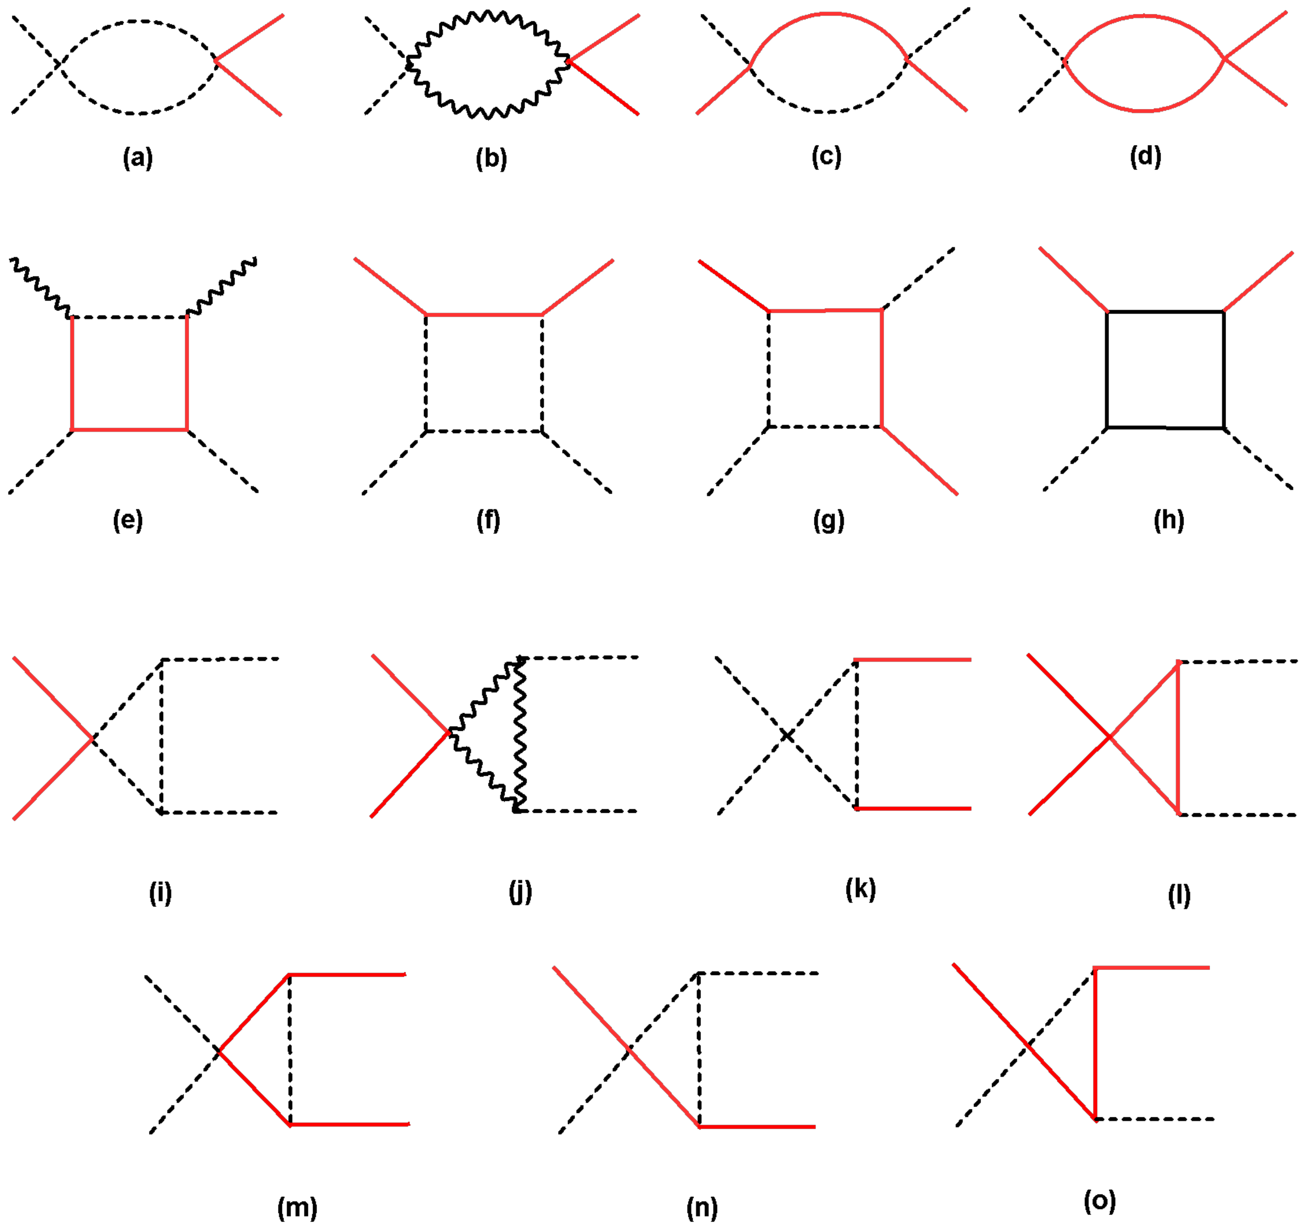


Figure 11: Feynman diagrams renormalizing quartic bosnic interaction $\lambda_{13}$ to the leading order.

The renormalization condition for $\lambda_{12}$ then reads as

$$\frac{1}{3}\, Z_{\Phi_1} Z_{\Phi_2} \lambda_{12,\mathrm{B}} - \mathrm{Con}^{(10)}_{(\mathrm{a})-(\mathrm{d})} - \mathrm{Con}^{(10)}_{(\mathrm{e})-(\mathrm{h})} - \mathrm{Con}^{(10)}_{(\mathrm{i})-(\mathrm{o})} = \lambda_{12,\mathrm{R}}, \tag{34}$$

from which we arrive at the RG flow equation for $\lambda_{12}$ quoted in the main part of the paper [see Eq. (6)].

• **Renormalization of** $\lambda_{13}$: The leading order renormalization of quartic bosonic coupling $\lambda_{13}$ arises from the Feynman diagrams shown in Fig. 11. The net contribution from diagrams (a)-(d) is given by

$$\mathrm{Con}^{(11)}_{(\mathrm{a})-(\mathrm{d})} = \left[\frac{1}{18}\left(N_b+2\right)\lambda_3\lambda_{13} + \frac{1}{6}\lambda_1\lambda_{13} + \frac{1}{18}\lambda_{12}\lambda_{23} + \frac{2}{9}\lambda_{13}^2\right] \frac{\Lambda^{D-4}}{8\pi^2}\, \ell. \tag{35}$$

The net contribution from diagrams (e)-(h) is given by

$$\mathrm{Con}^{(11)}_{(\mathrm{e})-(\mathrm{h})} = -8N_f g_1^2 g_3^2\, \frac{\Lambda^{D-4}}{8\pi^2}\ell + \left[8u_1^2u_3^2 + 8u_1u_3^3 + 8u_3^4\right] \frac{\Lambda^{D-8}}{8\pi^2}\, \ell. \tag{36}$$

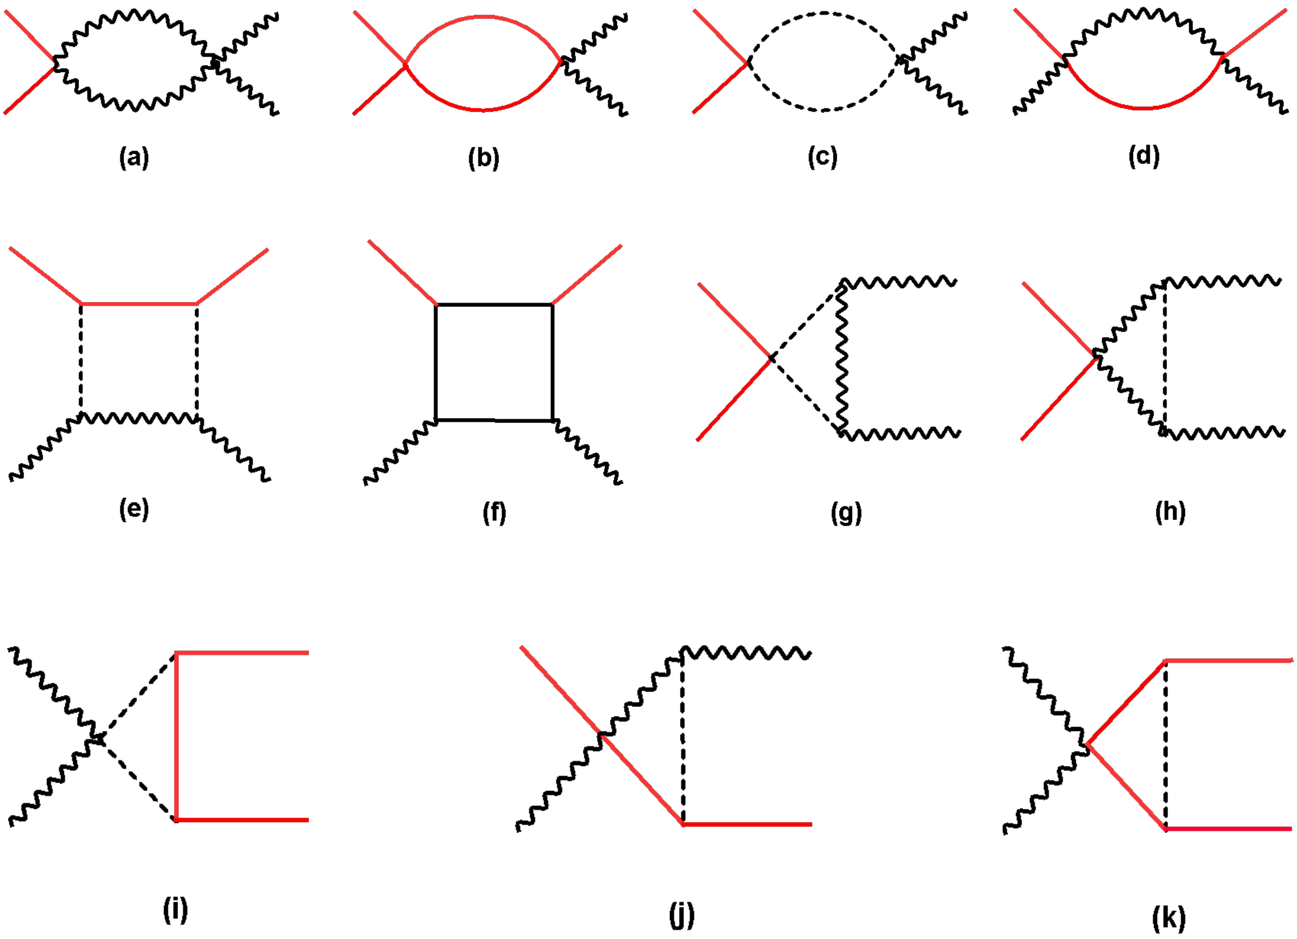


Figure 12: Feynman diagrams renormalizing quartic bosnic interaction $\lambda_{23}$ to the leading order.

The net contribution from diagrams (i)-(o) is given by

$$\mathrm{Con}^{(11)}_{(\mathrm{i})-(\mathrm{o})} = -\frac{2}{3}\left[\left(N_b+2\right)\lambda_3 u_3^2 + \lambda_{13} u_1^2 + \lambda_{23} u_2^2 + 3\lambda_1 u_3^2 + \lambda_{13} u_3^2 + 2\lambda_{13} u_1 u_3 + 2\lambda_{13} u_3^2\right] \frac{\Lambda^{D-6}}{8\pi^2}\,\ell. \tag{37}$$

The renormalization condition for $\lambda_{13}$ then reads as

$$\frac{1}{3}\, Z_{\Phi_1} Z_{\chi} \lambda_{13,\mathrm{B}} - \mathrm{Con}^{(11)}_{(\mathrm{a})-(\mathrm{d})} - \mathrm{Con}^{(11)}_{(\mathrm{e})-(\mathrm{h})} - \mathrm{Con}^{(11)}_{(\mathrm{i})-(\mathrm{o})} = \lambda_{13,\mathrm{R}}, \tag{38}$$

from which we arrive at the RG flow equation for $\lambda_{13}$ quoted in the main part of the paper [see Eq. (6)].

• **Renormalization of** $\lambda_{23}$: The leading order renormalization of quartic bosonic coupling $\lambda_{23}$ arises from the Feynman diagrams shown in Fig. 12. The net contribution from diagrams (a)-(d) is given by

$$\mathrm{Con}^{(12)}_{(\mathrm{a})-(\mathrm{d})} = \left[\frac{1}{6}\lambda_2\lambda_{23} + \frac{1}{18}\left(N_b+2\right)\lambda_3\lambda_{23} + \frac{2}{9}\lambda_{23}^2 + \frac{1}{18}\lambda_{12}\lambda_{13}\right] \frac{\Lambda^{D-4}}{8\pi^2}\,\ell. \tag{39}$$

The net contribution from diagrams (e) and (f) is given by

$$\mathrm{Con}^{(12)}_{(\mathrm{e})-(\mathrm{f})} = -24 N_f g_2^2 g_3^2 \,\frac{\Lambda^{D-4}}{8\pi^2}\,\ell + 8 u_3^2 u_2^2 \,\frac{\Lambda^{D-8}}{8\pi^2}\,\ell. \tag{40}$$

The net contribution from diagrams (g)-(k) is given by

$$\mathrm{Con}^{(12)}_{(\mathrm{g})-(\mathrm{k})} = -\left[\frac{2}{3}\lambda_{13} u_2^2 + \lambda_{23} u_2^2 + \frac{2}{3}\lambda_{12} u_3^2 + 2\lambda_{23} u_2 u_3 + \lambda_{23} u_3^2\right] \frac{\Lambda^{D-6}}{8\pi^2}\,\ell. \tag{41}$$

The renormalization condition for $\lambda_{23}$ then reads as

$$\frac{1}{3}\, Z_{\Phi_2} Z_{\boldsymbol{\chi}} \lambda_{23,\mathrm{B}} - \mathrm{Con}^{(21)}_{(\mathrm{a})-(\mathrm{d})} - \mathrm{Con}^{(12)}_{(\mathrm{e})-(\mathrm{f})} - \mathrm{Con}^{(12)}_{(\mathrm{g})-(\mathrm{k})} = \lambda_{23,\mathrm{R}}, \tag{42}$$

from which we arrive at the RG flow equation for $\lambda_{23}$ quoted in the main part of the paper [see Eq. (6)].
